# Supplementary material for: On the Inconsistency of Kernel Ridgeless Regression in Fixed Dimensions
Source: arXiv:2205.13525 source file (2023-04-12)
Supplement: Supplementary file 1 [file appendix_full.tex]

\section{Results for dimension greater than 1}
\label{sec:highd}

\subsection{Preliminaries}

$\Omega=(-\pi,\pi]^d$ and Kernel $k(x_1,x_2) = g(M_1((x_1-x_2)_1\mod\Omega), ..., M_d((x_1-x_2)_d\mod\Omega)) = g(\{M_i((\x_1-\x_2)_i\mod\Omega)\}_i)$. We will suppose $M_i = M$ for all $i \in [d]$. 

\begin{align}
    g(\{M_i((\x_1-\x_2)_i\mod\Omega)\}_i) &= \sum_{\k \in\Integer^d} G[\k]\exp(j\k \cdot (\x_1-\x_2))\\
    G[\k] &= \frac{1}{(2\pi)^d} \int_\Omega g(\{M_i(\x_i\mod\Omega)\}_i) \exp(-j \k \cdot \x)\dif \x
\end{align}

\begin{definition}
Let $X[\k]=X_{\k}=\mathcal{FS}\{x\}[\k]$ be the $\k$-th Fourier series coefficient of $x:\Omega \rightarrow \Real$, where $\k\in\Integer^d$.
\end{definition}

\begin{definition}[Circular Convolution in Higher Dimensions]
For $x,y:\Omega\rightarrow\Real$ we define the operator
\begin{align}
    (x\circconv^d y)(\t) = \int_{\Omega} x({\t}^\prime)y(\t-{\t}^\prime \mod \Omega)\dif{\t}^\prime
\end{align}
\end{definition}

\subsubsection{Assumptions}

\begin{definition}
Let $S_Q$ be the set of $\k \in \Integer^d$ such that $|k_i| \leq Q$ for all $i \in [d]$. Let $S^c_Q$ be the complement of this set (in the universe $\Integer^d$). 
\end{definition}

\begin{assumption}[Scale]
\label{ass:scale_highd}
$\displaystyle\sum_{\k \in \mathbb{Z}^d} |G[\k]| < \infty$ for all $M \geq 1$, $G[\k] = O_M(1)$ for all $\k \in \Integer^d$, and $G[\pmb{0}] = 1$. 
\end{assumption}

\begin{assumption}[Tail]
\label{ass:tail_highd}
$\displaystyle\sum_{\k \in S^c_{\ceil{M}^2}} G[\k] = O_M(1)$. 
\end{assumption}

\begin{assumption}[Head]
\label{ass:head_highd}
$\displaystyle\sum_{\k \in S_{\floor{M}}} G[\k] = \Theta_M(M^d)$.
\end{assumption}

\subsection{Noise-free estimation and approximation errors}

\begin{definition}
Let $\phi_k(x) = \frac{1}{\sqrt{2\pi}} e^{jkx}$ for $k\in\Integer$. In higher dimensions, $\phi_{\k}(\x) = \prod_{i=1}^d \phi_{k_i}(x_i)$.
\end{definition}

\begin{lemma}
\label{lemma:phi_mod_highd}
For $N$ evenly sampled points on the unit torus,
\begin{align*}
    {\phi_{\k}(x_n) = \phi_{\k \mod N}(x_n) = \phi_{k_1 \mod N}(x_{n,1}) \times \cdots \times \phi_{k_d \mod N}(x_{n,d})}
\end{align*} for $n \in [N]^d$, where $\k \mod N$, $\k\in\Integer^d$ acts component-wise. 
\end{lemma}

For a function $f^*\in L^2,$ define,
\begin{align}c_{\ell,f^*} = \frac{\sum_{\m \in \Integer^d} G[\m N + \ell] v_{\m N + \ell}}{\sum_{\m \in \Integer^d} (G[\m N + \ell])^2}, \qquad \ell\in[N]^d
\end{align}

\begin{lemma}
\label{lemma:orthogonal_comp_highd}
Let $f^* = \sum_{\k \in \Integer^d} v_{\k} \phi_{\k}$ for $\v_{k} \in \mathbb{R}$. We have, 
\begin{align}
    P_{\X}f^* = \frac{1}{(2\pi)^{d/2}} c_{\ell,f^*} \sum_{\m \in \Integer^d} G[\m N + \ell] e^{j(\m N + \ell)\cdot x} 
\end{align}
Further, \begin{align}
\|f^*-P_{\X}f^*\|^2_{L^2} = \sum_{\k \in \Integer^d} v^2_{\k} - \sum_{\ell \in [N]^d} \frac{\rbrac{\sum_{\m \in \Integer^d} G[\m N + \ell] v_{\m N + \ell}}^2}{\sum_{\m \in \Integer^d} (G[\m N + \ell])^2}.
\end{align}
\end{lemma}
\begin{proof}
Here we drop the subscript $L^2$ (all norms, inner products are $L^2$ unless specified otherwise). Let $\psi_{\ell}$ be a basis function for $\ell \in [N]^d$. As in $2$-d, because the span of the representers has $\frac{\psi_\ell}{\|\psi_\ell\|}$ as an orthonormal basis, we have \begin{align*}
    P_{\X}f^* &= \sum_{\ell \in [N]^d} \inner{f^*, \frac{\psi_\ell}{\|\psi_\ell\|}} \frac{\psi_\ell}{\|\psi_\ell\|}\\
    \norm{P_{\X}f^*}^2 &= \sum_{\ell \in [N]^d} \inner{f^*, \frac{\psi_\ell}{\|\psi_\ell\|}}^2
\end{align*} 

Let $\lambda_{\ell} = \prod_{i=1}^d \lambda_{\ell_i}$ Then,
\begin{align}
    \inner{f^*,\psi_{\ell}} = \sqrt{\frac{(2\pi N)^d}{\lambda_{\ell}}} \sum_{\m \in \Integer^d} G[\m N + \ell] v_{\m N + \ell} 
\end{align}
Recall from Lemma \ref{lem:psi_orthonormal_highd} that
\begin{align}
    \|\psi_{\ell}\|_{L^2} = \sqrt{\frac{(2\pi N)^d}{\lambda_\ell} \sum_{\m \in \Integer^d} \rbrac{G[\m N + \ell]}^2},\qquad \ell\in[N]^d. 
\end{align}
Then, for $\ell \in [N]^d$,
\begin{align}
    \inner{f^*, \frac{\psi_\ell}{\|\psi_\ell\|}} \frac{\psi_\ell}{\|\psi_\ell\|} &= \frac{1}{(2\pi)^{d/2}} \frac{\rbrac{\sum_{\m \in \Integer^d} G[\m N + \ell] e^{j(\m N + \ell)\cdot x} } \rbrac{\sum_{\m \in \Integer^d} G[\m N + \ell] v_{\m N + \ell}}}{\sum_{\m \in \Integer^d} (G[\m N + \ell])^2} \\
    &= \frac{1}{(2\pi)^{d/2}} c_{\ell,f^*} \sum_{\m \in \Integer^d} G[\m N + \ell] e^{j(\m N + \ell)\cdot x} 
\end{align}
The first claim follows.

For the second claim, we see that:
\begin{align}
    \norm{P_{\X}f^*}^2 &= \sum_{\ell \in [N]^d} \frac{(2\pi N)^d}{\lambda_{\ell}} \frac{1}{\|\psi_{\ell}\|^2} \rbrac{\sum_{\m \in \Integer^d} G[\m N + \ell] v_{\m N + \ell}}^2 \\ 
    &= \sum_{\ell \in [N]^d} \frac{\rbrac{\sum_{\m \in \Integer^d} G[\m N + \ell] v_{\m N + \ell}}^2}{\sum_{\m \in \Integer^d} (G[\m N + \ell])^2}
\end{align}
As $P_{\X}$ is the $L^2$ projection onto the span of the representers, the main lemma follows by the Pythagorean theorem.
\end{proof}

\begin{lemma}
Let $(f^* - P_{\X}f^*)_n$ be the vector of $f^* - P_{\X}f^*$ evaluated on the data with the same ordering as the kernel matrix $\Kmat$. Then,
\begin{align}
    \abs{ \K\inv(f^* - P_{\X}f^*)_n \cdot {\u}_{\k}}^2
    &= \frac{1}{(2\pi)^d} \rbrac{\frac{\sum_{\m \in \Integer^d} v_{\m M + \k}}{\sum_{\m \in \Integer^d} G[\m N + \k]} - \frac{\sum_{\m \in \Integer^d} G[\m N + \k] v_{\m N + \k}}{\sum_{\m \in \Integer^d} (G[\m N + \k])^2}}^2
\end{align}
\end{lemma}
\begin{proof}
Let $\beta_{\k,f^*} = \sum_{\m \in \Integer^d} v_{\m N + \k}$ for $\k \in [N]^d$.

By lemma \ref{lem:psi_orthonormal_highd}, lemma \ref{lemma:orthogonal_comp_highd}, and lemma \ref{lemma:phi_mod_highd}, we can write $Pf^*$ on a datapoint $x_{\p}$ with $\p \in [N]^d$ as
\begin{align}
    P_{\X}f^*(x_{\p}) = \frac{1}{(2\pi)^{d/2}} \sum_{\ell \in [N]^d} c_{\ell,f^*} \beta_{\ell,f^*} e^{j\ell \cdot x_{\p}} 
\end{align}
Then, where $\tilde{\beta} = ((\beta_{\ell} - c_{\ell,f^*} \|G_{\ell}\|_1)_{\ell \in [N]^d})\tran$, $\Lambda = (\lambda_{\ell})_{\ell}$, and $U$ is the $d$-dimensional DFT matrix (a $d$-fold Kronecker product of the $1$-d DFT matrix).
\begin{align}
    \Kmat\inv(f^* - Pf^*)_n \cdot u_k &= \frac{1}{(2\pi)^{d/2}} \rbrac{\Kmat\inv \rbrac{\sum_{\ell \in [N]^d} (\beta_{\ell,f^*} - c_{\ell,f^*} \|G_{\ell}\|_1) e^{j \ell \cdot x_{\p}}}_n }\tran v_k \\
    &= \frac{1}{(2\pi)^{d/2}} \rbrac{\Kmat\inv U \tilde{\beta}}\tran v_k \\
    &= \frac{1}{(2\pi)^{d/2}} \rbrac{U \Lambda^{-1} \tilde{\beta}}\tran v_k \\
    &= \frac{1}{(2\pi)^{d/2}} \tilde{\beta}^T \Lambda^{-1} U u_k \\
    &= \frac{1}{(2\pi)^{d/2}} \tilde{\beta}_k \lambda_k^{-1} \\
    &= \frac{1}{(2\pi)^{d/2}} \frac{\beta_{k} - c_{k,f} \|G_{k}\|_1}{\sum_{m \in \Integer} G[\m N + \k]} \\
    &= \frac{1}{(2\pi)^{d/2}} \frac{\sum_{\m \in \Integer^d} v_{\m M + \k} - \frac{\rbrac{\sum_{\m \in \Integer^d} G[\m N + \k]} \rbrac{\sum_{\m \in \Integer^d} G[\m N + \k] v_{\m N + \k}}} {\sum_{\m \in \Integer^d} (G[\m N + \k])^2}}{\sum_{\m \in \Integer^d} G[\m N + \k]} \\
    &= \frac{1}{(2\pi)^{d/2}} \rbrac{\frac{\sum_{\m \in \Integer^d} v_{\m M + \k}}{\sum_{\m \in \Integer^d} G[\m N + \k]} - \frac{\sum_{\m \in \Integer^d} G[\m N + \k] v_{\m N + \k}}{\sum_{\m \in \Integer^d} (G[\m N + \k])^2}}
\end{align}
\end{proof}

\begin{lemma}[MSE Expression (many dimensions)]
\label{lemma:MSE_highd}
\begin{align}
    &\Exp_\xi{\sbrac{\text{MSE}}} = \frac{1}{(2\pi)^d} \rbrac{\sum_{\k \in \Integer^d} v^2_{\k} - \sum_{\p \in [N]^d} \frac{\rbrac{\sum_{\m \in \Integer^d} G[\m N + \p] v_{\m N + \p}}^2}{\sum_{\m \in \Integer^d} (G[\m N + \p])^2}} \\
    &+ \frac{1}{(2\pi)^d} \sum_{\p \in [N]^d} \rbrac{\frac{\sum_{\m \in \Integer^d} v_{\m M + \p}}{\sum_{\m \in \Integer^d} G[\m N + \p]} - \frac{\sum_{\m \in \Integer^d} G[\m N + \p] v_{\m N + \p}}{\sum_{\m \in \Integer^d} (G[\m N + \p])^2} }^2 \sum_{\m \in \Integer^d} (G[\m N + \p])^2 \\
    & + \sigma^2 \sum_{\p \in [N]^d}  \frac{\sum_{\m \in \Integer^d} |G[\m N+\p]|^2}{\left|\sum_{\k \in \mathbb{Z}^d} G[\k N + \p] \right|^2}
\end{align}
\end{lemma}

\subsection{Theorem \ref{theorem:inconsistent_all_f} (many dimensions)}
\begin{lemma}
\label{lem:vanishing_tail_highd}
For kernel $g(\x)$ with $g : \Omega \rightarrow \Real$ that has a fixed bandwidth ($M$ does not vary with $N$) we have $\sum_{m \neq \pmb{0}} |G[\m N]| \rightarrow 0$ with $N \rightarrow 0$. 
\end{lemma}
\begin{proof}
The proof is similar to in $1$-d. Recall,
\begin{align}
    \sum_{\k \in \mathbb{Z}^d} |G[\k]| = O(M), \quad G[\pmb{0}] = 1
\end{align}
Therefore, where $S \subset \Integer^d$ is the set of $\k \in \Integer^d$ such that there exists $i \in [d]$ with $k_i \geq N$. Then, $\sum_{\k \in S} |G[\k]| \rightarrow 0$ with $N \rightarrow \infty$. The lemma follows, as ${\sum_{\k \in S} |G[\k]| \geq \sum_{m \neq \pmb{0}} |G[\m N]|}$. 
\end{proof}

\begin{theorem}[Inconsistency for all Functions ($d > 1$)]
Kernel interpolation with fixed bandwidth will be inconsistent for all functions in $L^1 \cap L^{\infty}$.
\end{theorem}
\begin{proof}
By lemma \ref{lemma:MSE_highd}, the estimation error is lower bounded by the first term ($\p=0$) in the sum. Further, we can apply lemma \ref{lem:vanishing_tail_highd} as in the 1-d case. 
\begin{align}
    \text{Estimation Error} &\geq \sigma^2 \frac{\sum_{\m \in \mathbb{Z}^d} |G^{M}[\m N]|^2}{\left|\sum_{\k \in \mathbb{Z}^d} G^{M}[(\k_i N +\p_i)_{i=1}^d]\right|^2} \\
    &\geq \sigma_2 \frac{(G[\pmb{0}])^2 + o(1)}{(G[\pmb{0}] + o(1))^2} \\
    &\geq \Omega(\sigma^2)
\end{align}

% By lemma \ref{lem:vanishing_tail}, 
% \begin{align}
%     \Exp_{\xivec} \left[ \frac{1}{(2\pi)^d} \int_\Omega |f(\t) - \widehat{f}(\t)|^2 \dif \t \right] &\geq \sigma^2 \frac{|G^{M}[\pmb{0}]|^2 + o(1)}{|G^{M}[\pmb{0}]|^2 + o(1) + O(|G^{M}[\pmb{0}]|) \sum_{\k \neq \pmb{0}} |G^{M}[\k N]| + o(1)} \\
%     &= \sigma^2 \frac{|G^{M}[\pmb{0}]|^2 + o(1)}{|G^{M}[\pmb{0}]|^2 + o(1) + o(1)}
% \end{align}
% As $|G^{M}[\pmb{0}]|^2 = \Omega(1)$, we have the main theorem. 
\end{proof}

% \subsection{Vanishing Estimation Error}

% We can upper bound the estimation error in the sum from Theorem \ref{thm:MSE_highd}. In particular, the theorem states:
% \begin{align}
%     \text{Estimation Error} = \sigma^2 \sum_{\p \in [N]^d} \sum_{\m \in \Integer^d} \frac{|G[\m N+\p]|^2}{\left|\sum_{\k \in \mathbb{Z}^d} G[\k N + \p] \right|^2}
% \end{align}
% To get vanishing estimation error it is sufficient to show each one of terms is strictly smaller than $N^{-d}$. 

% Consider a single term $\p \in [N]^d$. Then, for $M=N^2$,
% \begin{align}
%     \sum_{\m \in \Integer^d} \frac{|G[\m N+\p]|^2}{\left|\sum_{\k \in \mathbb{Z}^d} G[\k N + \p] \right|^2} &= \frac{O(N^{d})}{\Theta(N^{2d})} = O(N^{-d})
% \end{align}
% As there are $N^d$ such terms, this proves the theorem.

\subsection{Theorem \ref{theorem:inconsistent_all_band} (many dimensions)}

\subsection{Higher, but fixed dimensions}

\begin{theorem}[Parseval's theorem in high dimensions]
\label{thm:highd_parseval_continuous}
For a $2\pi$-periodic signal $f(\t)$ in $d$ dimensions with Fourier series coefficients $c_{\k}$ for $k \in \Integer^d$, we have
\begin{align}
    \sum_{\k \in \Integer^d} |c_{\k}|^2 = \frac{1}{(2\pi)^d} \int_\Omega |f(\t)|^2 \dif \t
\end{align}
\end{theorem}

\begin{lemma}[Convolution is multiplication in high-$d$ Fourier domain]
\label{lemma:highd_conv_omega}
    Suppose $2\pi$-perioidic signals $x,y: \Omega \rightarrow \Real$ have Fourier series coefficients $X[\k],Y[\k]$ respectively for $\k \in \Integer^d$. Then, 
    \begin{align}
        \mathcal{FS}\{x \circconv^d y\}[\k] = (2\pi)^d X[\k] Y[\k] 
    \end{align}
\end{lemma}
\begin{proof} 
It suffices to show that $(x\circconv^d y)(t)=\sum_{\k \in\Integer^d}X_{\k} Y_{\k} \exp(j\k \cdot t)$. Now consider,
\begin{align}
    x(t) &= \sum_{\k \in\Integer^d} X_{\k} \exp(j\k \cdot t)\qquad
    y(t) = \sum_{\k \in\Integer^d} Y_{\k} \exp(j\k \cdot t)\\
    (x\circconv^d y)(t) &= \int_\Omega x(\tau) y(t-\tau \mod \Omega)\dif\tau\\
    &= \int_\Omega \rbrac{\sum_{\k \in\Integer^d} X_{\k} \exp(j \k \cdot \tau) }
    \rbrac{\sum_{\k^\prime \in\Integer^d} Y_{\k^\prime} \exp(j\k^\prime \cdot (t-\tau \mod \Omega))}\dif\tau\\
    &=\sum_{\k,\k^\prime\in\Integer}  X_{\k} Y_{\k^\prime} \int_\Omega    \exp(j\k \cdot \tau)  \exp(j\k^\prime \cdot (t-\tau \mod \Omega))\dif\tau\qquad\{t-\tau\longleftarrow u\}\\
    &=\sum_{\k,\k^\prime\in\Integer^d}  X_{\k} Y_{\k^\prime}\int_\Omega\exp(j\k \cdot (t-u)+j\k^\prime \cdot (u \mod \Omega))\dif u\\
    &=\sum_{\k,\k^\prime\in\Integer^d} X_{\k} Y_{\k}\exp(j\k \cdot t)\mathbf{1}_{\{\k=\k^\prime\}}\cdot (2\pi)^d
    =\sum_{\k \in\Integer^d}X_{\k} Y_{\k} \exp(j\k \cdot t)\cdot (2\pi)^d
\end{align}
which concludes the proof.
\end{proof}

\subsubsection{Approximation error lemmas}

\begin{lemma}[Eigenvectors of $\Kmat$ ($d > 1$)]\label{lem:eigenvectors_of_Kmat_highd}
The eigenvectors for $\Kmat$ are $\bar{u}_{\ell} = \{e^{-j \ell \cdot \x_{\p}}\}_{\p}$ for $\ell \in [N]^d$ with eigenvalues 
\begin{align}
N^d \lambda_\ell = N^d \sum_{\m \in \Integer^d} G[\m N + \ell].    
\end{align}
\end{lemma}

\begin{proof}[Proof of \Cref{lem:eigenvectors_of_Kmat_highd}]
\begin{subequations}
Let $i \in [N]^d$
\begin{align}
    (\Kmat v_{\ell})_{i} = \sum_{\p \in [N]^d} \Kmat_{i,\p} v_{\ell \p} &= \sum_{\p} \sum_{\m \in \Integer^d} G[\m] e^{j \frac{2\pi \m \cdot (i - \p)}{N}} e^{\frac{j 2\pi \p \cdot \ell }{N}} \\
    &= \sum_{\m \in \Integer} G[\m] e^{j \frac{2\pi \m \cdot i}{N}} \sum_{\p \in [N]^d}  e^{j \frac{2\pi (\ell-\m)\cdot \p}{N}} \\
    &= N^d \sum_{\m \in \Integer} G[\m N + \ell] e^{j \frac{2\pi (\m N + \ell) \cdot i}{N}} \\
    &= e^{j \frac{2\pi \ell \cdot i}{N}} N^d \sum_{m \in \Integer} G[mN + \ell] e^{j \frac{2\pi N \m \cdot i}{N}} \\
    &= e^{j \frac{2\pi \ell \cdot i}{N}} N^d \sum_{m \in \Integer} G[\m N + \ell] \\
    &= e^{j \frac{2\pi \ell \cdot i}{N}} N^d \lambda_\ell
\end{align}
\end{subequations}
\end{proof}

\begin{lemma}[Eigenfunctions of $\Kcov$ ($d > 1$)]\label{lem:eigenfunctions_of_Kcov_highd}
The eigenfunctions for the empirical kernel transform $\Kcov$ are,
\begin{align}
    \psi_\ell(x) &= \sqrt{\frac{N^d}{\lambda_\ell}} \sum_{\m \in \Integer} G[\m N + \ell] e^{j (\m N + \ell) \cdot x},\qquad \ell\in[N]^d.
\end{align}
\end{lemma}
\begin{proof}[Proof of Lemma \ref{lem:eigenfunctions_of_Kcov_highd}]
As in the $1$-d case, by Lemma \ref{lemma:eigvectors_covariance}, we have
\begin{align}
    \psi_{\ell}(x) &= \inner{\frac{(e^{-j \ell \cdot \x_{\p}})_n}{\sqrt{N^d \lambda_{\ell}}}, K(X_N)}_n (x) \\
    &= \frac{1}{\sqrt{N^d \lambda_{\ell}}} \sum_{\p \in [N]^d} K(x,x_{\p}) e^{j \frac{2\pi \ell \cdot \p}{N}} \\
    &= \frac{1}{\sqrt{N^d \lambda_{\ell}}} \sum_{\p \in [N]^d} \sum_{\m \in \Integer^d} G[\m] e^{j\m \cdot x} e^{-j \frac{2\pi \m \cdot \p}{N}} e^{j \frac{2\pi \ell \cdot \p}{N}} \\
    &= \frac{1}{\sqrt{N^d \lambda_{\ell}}} \sum_{\m \in \Integer^d} G[\m] e^{j\m \cdot x} \sum_{n=1}^N  e^{-j \frac{2\pi (\m-\ell) \cdot \p}{N}} \\
    &= \frac{N^d}{\sqrt{N^d \lambda_{\ell}}} \sum_{\m \in \Integer^d} G[\m] e^{j\m \cdot x} \mathbbm{1}\{\m - \ell \in N \cdot \Integer\} \\
    \implies \psi_{\ell}(x) &= \sqrt{\frac{N^d}{\lambda_{\ell}}} \sum_{\m \in \Integer} G[\m N + \ell] e^{j (\m N + \ell) \cdot x}
\end{align}
\end{proof}

\begin{lemma}
\label{lem:psi_orthonormal_highd}
The eigenfunctions $\psi_\ell$ (for $\ell \in [N]^d$) are orthogonal in $L^2$ (i.e. $\inner{\psi_\ell, \psi_{k}}_{L^2} = 0$ for $\k \neq \ell$). Let $\lambda_{\ell} = \prod_{i=1}^d \lambda_{\ell_i}$. Further, the eigenfunctions $\psi_\ell$ have norm 
\begin{align}
\|\psi_{\ell}\|_{L^2}^2 = \frac{(2\pi N)^d}{\lambda_\ell} \sum_{m \in \Integer^d} \rbrac{G[\m N + \ell]}^2,\qquad \ell\in[N]^d.    
\end{align}
\end{lemma}
\begin{proof}[Proof of \Cref{lem:psi_orthonormal_highd}]
Suppose $\k \neq \ell$.
\begin{align}
    \inner{\psi_{\ell},\psi_k} &= \sqrt{\frac{N^{2d}}{\lambda_{\ell}\lambda_k}} \sum_{\m,\m^\prime \in \Integer^d} G[\m N + \ell] G[\m^\prime N + \k] \inner{e^{j(\m N + \ell) \cdot x},e^{j(\m N + \k) \cdot x}}_{L^2} \\
    &= 0 
\end{align}
For the second claim,
\begin{align}
\inner{\psi_{\ell}, \psi_{\ell}}_{L^2} &= \frac{N^d}{\lambda_{\ell}} \sum_{\m \in \Integer^d} \rbrac{G[\m N + \ell]}^2 \|e^{j(\m N + \ell) \cdot x}\|_{L^2} \\
&= \frac{(2\pi N)^d}{\lambda_{\ell}} \sum_{\m \in \Integer^d} \rbrac{G[\m N + \ell]}^2
\end{align}
\end{proof}
