# Supplementary material for: On the Inconsistency of Kernel Ridgeless Regression in Fixed Dimensions
Source: arXiv:2205.13525 source file (2023-04-12)
Supplement: Supplementary file 3 [file old_appendix.tex]

\section{Old stuff}
\begin{lemma}
For the DFT on the $N$ samples of the unit circle. 
\begin{align}
     \Exp \left| [\mathcal{F}]\left(f - \widehat{f}\right)(\omega) \right|^2 = |G(\omega)|^2 \cdot \trace \left( \K^{-2} (e^{i\omega},...,e^{i\omega N})\herm (e^{-i\omega},...,e^{-i\omega N}) \right)
\end{align}
\end{lemma}
\begin{proof}
Let $\widehat{u}$ be the discrete time Fourier transform of a signal $u$. As $y_0 = K \alpha^*$ and $y = y_0 + \xi$,
\begin{align*}
    \widehat{\alpha}(\omega) = \sum_{n=1}^N \alpha[n] e^{-j \omega N} &= (K^{-1}y) \cdot  (e^{-j \omega},...,e^{-j \omega N}) \\
    &= (\alpha^* + K^{-1}\xi) \cdot  (e^{-j \omega},...,e^{-j \omega N})
\end{align*}
for $w\in[-\pi,\pi).$ Then,
\begin{align*}
    \widehat{\alpha}(\omega) &= \alpha^*\cdot  (e^{-j \omega},...,e^{-j \omega N}) + (K^{-1}\xi) \cdot  (e^{-j \omega},...,e^{-j \omega N}) \\
    &= \widehat{\alpha^*}(\omega) + (K^{-1}\xi) \cdot  (e^{-j \omega},...,e^{-j \omega N}) \\
    &= \widehat{\alpha^*}(\omega) + \sum_{n=1}^N \left(\sum_{n^\prime=1}^N K^{-1}(n^\prime,n) \xi_{n^\prime} \right) e^{-j \omega N}
\end{align*}

Then, the discrete time FT of $f - \hat{f}$ can be written as the following, where $G$ is the Fourier transform of $g(x-y) = k(x,y)$,
\begin{align*}
    [\mathcal{F}]\left(f - \widehat{f}\right)(\omega) &=  \widehat{\alpha^*}(\omega) G(\omega) - \left(\widehat{\alpha^*}(\omega) + (e^{-j \omega},...,e^{-j \omega N}) \cdot K^{-1}\xi \right) G(\omega) \\
    &= \left((e^{-j \omega},...,e^{-j \omega N}) \cdot \K\inv \xi\right) G(\omega)
\end{align*}
Therefore, 
\begin{align*}
    \Exp \left| [\mathcal{F}]\left(f - \widehat{f}\right)(\omega) \right|^2 &= |G(\omega)|^2 \cdot \Exp \left[\left( \sum_{n,n^\prime} \K\inv(n,n^\prime) \xi_{n^\prime} e^{-j \omega N} \right) \left( \sum_{n,n^\prime} \K\inv(n,n^\prime) \xi_{n^\prime} e^{+j \omega N} \right)\right] \\
    &= |G(\omega)|^2 \cdot \sum_{n^\prime}^N \sum_{n,m} K^{-1}(n,n^\prime) K^{-1}(n^\prime,m) e^{-j(n-m)w} \\ 
    &= |G(\omega)|^2 \cdot \sum_{n,m} K^{-2}(n,m) e^{-j(n-m)w} \\
    &= |G(\omega)|^2 \cdot \trace \left( \K^{-2} (e^{i\omega},...,e^{i\omega N})\herm (e^{-i\omega},...,e^{-i\omega N}) \right)
\end{align*}
\end{proof}

\begin{remark}[Sample MSE]
\label{rem:sample_mse}
Note that for the Rademacher noise model, 
\begin{align}
    \sum_{\omega \in \{\frac{2\pi}{N},...,2\pi\}} \Exp \left| [\mathcal{F}]\left(f - \widehat{f}\right)(\omega) \right|^2 = N \sum_{i=1}^N \Exp \left(f(x_i) - \widehat{f}(x_i) \right)^2 = N \sum_{i=1}^N \Exp \xi^2_i = N^2
\end{align}
\end{remark}

\subsection{Continuous Fourier Transform}

Quite clearly the error on the sample of an interpolating kernel ridge regression will have MSE of $1$. We will show now that the MSE on the population under the assumptions of the previous section (i.e. that the target function is in the span of the representers) is equal to the MSE on the sample.

To do this, we will analyze the Fourier transform of the continuous signals $f(x)$ and $\hat{f}(x)$. We begin by noting,
\begin{align}
    \hat{f}(x) = \sum_{i=1}^N \alpha_i k(x - x_i) &= \sum_{i=1}^N \alpha_i \int_{-\infty}^\infty k(x^\prime - x) \delta(x^\prime - x_i) dx^\prime \\
    &= \sum_{i=1}^N \int_{-\infty}^\infty k(x^\prime - x) \alpha(x^\prime) \delta(x^\prime - x_i) dx^\prime \\
    &= \sum_i (\alpha\delta_{x_i} * k)(x) 
\end{align}
Further,
\begin{align}
    f(x) = \sum_i (\alpha^* \delta_{x_i} * k)(x) 
\end{align}
So, where $G_c(\omega)$ is the continuous-time fourier transform of $g(x-y) = k(x,y)$,
\begin{align}
    [\mathcal{F}](\hat{f} - f)(\omega) &= \sum_i \alpha(x_i) e^{-i\omega x_i}G_c(\omega) - \sum_i \alpha^*(x_i) e^{-i\omega x_i}G_c(\omega) \\
    &= (\alpha - \alpha^*) \cdot (e^{-i\omega x_1},...,e^{-i\omega x_N}) G_c(\omega) \\
    &= (\K\inv \xi) \cdot (e^{-i\omega x_1},...,e^{-i\omega x_N}) G_c(\omega)
\end{align}
Suppose the data are drawn from the grid as in Section \ref{sec:unit_circle}. Then,
\begin{align}
    \mathbb{E}\left|[\mathcal{F}](\hat{f} - f)(\omega)\right|^2 &= \mathbb{E}\left[|G_c(\omega)|^2 |(\K\inv \xi) \cdot (e^{-i\omega x_1},...,e^{-i\omega x_N})|^2 \right] \\
    &= |G_c(\omega)|^2 \trace(\K^{-2} (e^{i\omega},...,e^{i\omega N})\herm (e^{-i\omega},...,e^{-i\omega N}))
\end{align}
Note as the kernel function $g$ is perioidic, its CTFT is a Fourier series - i.e. a sequence of impulses at the Fourier coefficients of $g$ (multiplied by a factor of $N$). Further, the coefficients of the continuous time signal $g$ take the following form:
\begin{align}
    c_k = \frac{1}{2\pi} \int_{0}^{2\pi} g(t) e^{-ikt} \dif t
\end{align}
Further, by \url{https://math.stackexchange.com/questions/569750/speed-of-convergence-of-riemann-sums},
\[
  |G_c(\omega) - G(\omega)| = 
  \begin{cases}
        O\left(\frac{\max{t}  {g(t)}}{N} \right) & \text{if $\omega = \frac{2\pi k}{N}$} \\
        0 & \text{o.w.}
  \end{cases}
\]

Parseval's Power Theorem says that the MSE of the whole signal \url{https://www.tutorialspoint.com/signals-and-systems-parseval-s-power-theorem} is equal to the squared sum of the Fourier Coefficients (which is $N^2$ times the energy of the DFT). Therefore,
\begin{align}
    2\pi N^2 \text{MSE}_c[f - \hat{f}] &= \int_{\omega \in [0,2\pi)} |\text{\{CTFT\}}(f - \hat{f})|^2 = \sum_{\omega \in \{\frac{2\pi}{N}, ..., 2\pi\}} |\text{\{DTFT\}}(f - \hat{f})|^2 = N^2 \\
    \implies \text{MSE}_c[f - \hat{f}] &= \frac{1}{2\pi}
\end{align}

\subsection{Distance to the Span of the Kernels}

We now relax the assumption that the target function is in the span of the represeneters for the data. In particular, where $\Pi_{\X}$ is the projection operator onto the span of the representers and $f_{\perp}$ is the component of $f$ perpendicular to the span, we can decompose the target function as
\begin{align}
    f(x) &= \Pi_{\X}(f)(x) + f_{\perp}(x) \\
    &= \sum_{n=1}^N \alpha^*_n k(x,x_n) + f_{\perp}(x) \\
    &= k(x,\X)^\top \alpha^* + f_{\perp}(x)
\end{align}
In this case, $y = \K\alpha^* + f_{\perp}(\X) + \xi$, and so
\begin{align}
    \hat{f}(x) &= \sum_{n=1}^N \alpha_n k(x,x_n) \\
    &= \alpha^\top k(x,\X) \\
    &= k(x,\X)^\top \K\inv\left(\K\alpha^* + f_{\perp}(\X) + \xi\right)  \\
    &= k(x,\X)^\top \left( \alpha^*  + \K\inv f_{\perp}(\X) + \K\inv\xi \right) \\
    &= k(x,\X)^\top \alpha^* + k(x,\X)^\top \left(\K\inv f_{\perp}(\X) + \K\inv\xi \right)
\end{align}

\subsection{Relaxed DFTF}
For $w\in[-\pi,\pi).$
\begin{align*}
    \widehat{\alpha}(\omega) = \sum_{n=1}^N \alpha[n] e^{-j \omega N} &= (\alpha^* + \K\inv\xi + \K\inv f_{\perp}(\X)) \cdot  (e^{-j \omega},...,e^{-j \omega N}) \\
    &= \alpha^*\cdot  (e^{-j \omega},...,e^{-j \omega N}) + (\K\inv \xi) \cdot  (e^{-j \omega},...,e^{-j \omega N}) + (\K\inv f_{\perp}(\X)) \cdot (e^{-j \omega},...,e^{-j \omega N}) \\
    &= \widehat{\alpha^*}(\omega) + (\K\inv\xi) \cdot  (e^{-j \omega},...,e^{-j \omega N}) + (\K\inv f_{\perp}(\X)) \cdot (e^{-j \omega},...,e^{-j \omega N})\\
    &= \widehat{\alpha^*}(\omega) + \sum_{n=1}^N \left(\sum_{n^\prime=1}^N \K\inv(n^\prime,n) \xi_{n^\prime} \right) e^{-j \omega N} + (\K\inv f_{\perp}(\X)) \cdot (e^{-j \omega},...,e^{-j \omega N})
\end{align*}

Therefore, 
\begin{align*}
    \Exp \left| [\mathcal{F}]\left(f - \widehat{f}\right)(\omega) \right|^2 &= \Exp \Bigg[\left( G(\omega)\sum_{n,n^\prime} \K\inv(n,n^\prime) \xi_{n^\prime} e^{-j \omega N} +  G(\omega)\K\inv f_{\perp}(\X) \cdot (e^{-j \omega},...,e^{-j \omega N}) - \mathcal{F} f_{\perp}(\omega) \right) \\
    &\left( \overline{G(\omega)}\sum_{n,n^\prime} \K\inv(n,n^\prime) \xi_{n^\prime} e^{j \omega N} + \overline{G(\omega)}\K\inv f_{\perp}(\X) \cdot (e^{j \omega},...,e^{j \omega N}) - \overline{\mathcal{F} f_{\perp}(\omega)}\right)\Bigg] \\
    &= |G(\omega)|^2 \sum_{n^\prime}^N \sum_{n,m} K^{-1}(n,n^\prime) K^{-1}(n^\prime,m) e^{-j(n-m)w} \\ 
    &+ \left|G(\omega) \K\inv f_{\perp}(\X) \cdot (e^{-j \omega},...,e^{-j \omega N}) - \mathcal{F} f_{\perp}(\omega)\right|^2 \\~\\
    %
    &= |G(\omega)|^2 \cdot \sum_{n,m} K^{-2}(n,m) e^{-j(n-m)w} \\
    &+ \left|G(\omega) \K\inv f_{\perp}(\X) \cdot (e^{-j \omega},...,e^{-j \omega N}) - \mathcal{F} f_{\perp}(\omega)\right|^2\\~\\
    %
    &= |G(\omega)|^2 \cdot \trace \left( \K^{-2} (e^{i\omega},...,e^{i\omega N})\herm (e^{-i\omega},...,e^{-i\omega N})\right) \\ 
    &+ \left|G(\omega) \K\inv f_{\perp}(\X) \cdot (e^{-j \omega},...,e^{-j \omega N}) - \mathcal{F} f_{\perp}(\omega)\right|^2 \\~\\
    %
    &= |G(\omega)|^2 \cdot \trace \left( \K^{-2} (e^{i\omega},...,e^{i\omega N})\herm (e^{-i\omega},...,e^{-i\omega N})\right) \\ 
    &+ \left|G(\omega) \K\inv f_{\perp}(\X) \cdot (e^{-j \omega},...,e^{-j \omega N}) - \mathcal{F} f_{\perp}(\omega)\right|^2 \\
\end{align*}

\subsection{Relaxed CTFT}

Where $G_c(\omega)$ is the continuous-time fourier transform of $g(x-y) = k(x,y)$,
\begin{align}
    [\mathcal{F}](\hat{f} - f) &= \sum_i \alpha(x_i) e^{-i\omega x_i}G_c(\omega) - \sum_i \alpha^*(x_i) e^{-i\omega x_i}G_c(\omega) - \mathcal{F} f_{\perp}(\omega) \\
    &= (\alpha - \alpha^*) \cdot (e^{-i\omega x_1},...,e^{-i\omega x_N}) G_c(\omega) - \mathcal{F} f_{\perp}(\omega)\\
    &= (\K\inv \xi + \K\inv f_{\perp}(\X) ) \cdot (e^{-i\omega x_1},...,e^{-i\omega x_N}) G_c(\omega) - \mathcal{F} f_{\perp}(\omega)
\end{align}
Suppose the data are drawn from the grid as in Section \ref{sec:unit_circle}. Then, as the cross terms are $0$ in expectation,
\begin{align}
    \mathbb{E}\left|[\mathcal{F}](\hat{f} - f)\right|^2 &= \mathbb{E}\left[|G_c(\omega)|^2 |(\K\inv \xi) \cdot (e^{-i\omega x_1},...,e^{-i\omega x_N})|^2 \right] + \left|G_c(\omega)(\K\inv f_{\perp}(\X)) \cdot (e^{-i\omega x_1},...,e^{-i\omega x_N}) - \mathcal{F} f_{\perp}(\omega)\right|^2\\
    &= |G_c(\omega)|^2 \trace(\K^{-2} (e^{i\omega},...,e^{i\omega N})\herm (e^{-i\omega},...,e^{-i\omega N})) \\
    &+ \left|G_c(\omega)(\K\inv f_{\perp}(\X)) \cdot (e^{-i\omega x_1},...,e^{-i\omega x_N}) - \mathcal{F} f_{\perp}(\omega)\right|^2\\
\end{align}

Applying Parseval's theorem in the discrete and continous cases,
\begin{align}
    2\pi N^2 \text{MSE}_c[f - \hat{f}] &= \int_{\omega \in [0,2\pi)} |\text{\{CTFT\}}(f - \hat{f})|^2 = \sum_{\omega \in \{\frac{2\pi}{N}, ..., 2\pi\}} |\text{\{DTFT\}}(f - \hat{f})|^2 = N^2 \\
    \implies \text{MSE}_c[f - \hat{f}] &= \frac{1}{2\pi}
\end{align}

\section{Computing the Trace}
We'll compute the case in the setting from Section \ref{sec:unit_circle}. In particular, by lemma \ref{lemma:kernel_unit_circle}, the Kernel inverse there has the form $\K\inv = \frac1n\sum_{\ell\in[n]} \frac1{\gamma[\ell]}\v_\ell\v_\ell\herm$ where $\gamma = \sum_{m\in\Integer}\beta[mn+\ell]$ and $\v_\ell=\begin{bmatrix}1 & \exp(j\tfrac{2\pi}{n}\ell) & \exp(j\tfrac{2\pi}{n}2\ell) & \ldots & \exp(j\tfrac{2\pi}{n}(n-1)\ell)\end{bmatrix}\T$. Note this is an eigen-decomposition of $\K\inv$ and so we can write $\K^{-2} = \frac1{n^2}\sum_{\ell\in[n]} \frac1{\gamma^2[\ell]}\v_\ell\v_\ell\herm$. Let $g(\theta) = \sum_k \beta[k] e^{j \omega\theta}$ be the Fourier series representation of $g$. Because $g$ is periodic, its Fourier transform has the following form (see e.g. \url{http://dsp.cs.cmu.edu/notes/dtft/dtft.html#dtft}), where $\omega \in [0,2\pi]$,

\[
  G(\omega) =
  \begin{cases}
        \beta[k] & \text{if $\omega = \frac{2\pi k}{n}$} \\
        0 & \text{o.w.}
  \end{cases}
\]

Further, $\trace \left( \K^{-2} e^{-j[n]w}(e^{-j[n]w})^H \right) = \frac{1}{n^2} \frac{1}{\gamma^2[k \mod n]}$ for $\omega = \frac{2\pi k}{n}$, as
\begin{align}
    \K^{-2} (1,...,e^{-j(n-1)\omega})^T (1,...,e^{j(n-1)\omega}) &= \frac{1}{n^2} \sum_{\ell=0}^{n-1} \frac{1}{\gamma^2[\ell]} \v_\ell \v_\ell\herm \v_k \v_k\herm  \\
    &= \frac{1}{n^2} \frac{1}{\gamma^2[k \mod n]} \v_k \v_k\herm
\end{align}
Note that $\trace(\v_k \v_k\herm)= 1$. Therefore, applying Parseval's theorem,
\begin{align}
    \mathbb{E}[MSE] = \sum_{\omega = \frac{2\pi k}{n}} \Exp \left| [\mathcal{F}]\left(f - \widehat{f}\right)(\omega) \right|^2  &= \sum_{\omega = \frac{2\pi k}{n}}  \left|G(\omega) \right|^2 \trace \left( \K^{-2} e^{-j[n]w}(e^{-j[n]w})^H \right) \\ 
    %
    &= \frac{1}{n^2}  \sum_{k \in [n]} \frac{|G(\frac{2\pi k}{n})|^2}{\gamma^2[k \mod n]}\\
    %
    &= \sum_{k \in [n]} \left(\frac{\beta[k]}{\gamma[k \mod n]}\right)^2
\end{align}



\subsection{Lower bound}

Suppose $\beta(k) = e^{-|k|}$. We derived for uniform data on the unit circle that the expected error is equal to
\begin{align}
    &\sum_{k \in \mathbb{Z}} \left( \frac{\beta[k]}{\sum_{m \in \mathbb{Z}} \beta[mn + k \mod n]}\right)^2  \geq \sum_{0\leq k \leq n/6} \left( \frac{\beta(k)}{\sum_{m \in \mathbb{Z}} \beta[mn + k \mod n]}\right)^2 \\
    &= \sum_{0\leq k \leq n/6} \left( \frac{\beta[k]}{\beta[k] + \sum_{m \in \mathbb{Z}^*} \beta[mn + k \mod n]}\right)^2\\
    &= \sum_{0\leq k \leq n/6}  \frac{\beta^2[k]}{\beta^2[k] + 2\beta[k] \cdot \sum_{m \in \mathbb{Z}^*} \beta[mn + k \mod n] + (\sum_{m \in \mathbb{Z}^*} \beta[mn + k \mod n])^2} \\
    &= \sum_{0\leq k \leq n/6}  \frac{\beta^2[k]}{\beta^2[k] + 2\beta^2[k] \cdot \sum_{m \in \mathbb{Z}^+} \beta[mn] + 2\beta[k]\beta[n-k] \cdot \sum_{m \in \mathbb{Z}^+} \beta[mn] + (\sum_{m \in \mathbb{Z}^*} \beta[mn + k \mod n])^2} \\
    &\geq \sum_{0\leq k \leq n/6}  \frac{\beta^2[k]}{\beta^2[k] + 2\beta^2[k] \cdot \sum_{m \in \mathbb{Z}^*} \beta[mn] + (\beta[k] \sum_{m \in \mathbb{Z}^+} \beta[mn] + \beta[n-k] \sum_{m \in \mathbb{Z}^+} \beta[mn])^2} \\
    &\geq \sum_{0\leq k \leq n/6}  \frac{\beta^2[k]}{\beta^2[k] + 2\beta^2[k] \cdot \sum_{m \in \mathbb{Z}^*} \beta[mn] + 4\beta^2[k]( \sum_{m \in \mathbb{Z}^+} \beta[mn])^2} \\
    &= \sum_{0\leq k \leq n}  \frac{\beta^2[k]}{\beta^2[k] + 2e^{-2k} \cdot O(e^{-n}) + e^{-2k} O(e^{-n})^2} \\
    &= \sum_{0\leq k \leq n/6}  \frac{\beta^2[k]}{\beta^2[k] + O(e^{-n})} \\
    &= n/6 - \sum_{0\leq k \leq n/6}  \frac{O(e^{-n})}{\beta^2[k] + O(e^{-n})} \\
    &\geq n/6 - O(e^{-n}) \sum_{0\leq k \leq n/6}  \frac{1}{\beta^2[k]} \\
    &= n/6 - O(e^{-n}) O(e^{n/3})
\end{align}

A similar argument holds for the Gaussian tail where $\beta(k) = e^{-k^2}$.

\subsection{Littlewood stuff}

As the normalized kernel is singular (or approximately so), the inverted matrix is approximately identity ${(K \approx K^{-1} \approx I)}$. Then, for $z_n = e^{-j \omega N}$,

\begin{align*}
    \widehat{\alpha}(\omega) &= \widehat{\alpha^*}(\omega) + \sum_{n=1}^N  \xi_n e^{-j \omega N}
\end{align*}

This what is called a Littlewood polynomial. We recall the following lemma introduced by 
Littlewood and Offord \cite{littlewoodofford1938} 
and improved by Erdös \cite{erdos1943} regarding 
the anticoncentration of these polynomials.

\begin{lemma}[Anticoncentration of Littlewood 
Polynomials \cite{erdos1943}]
    Suppose we are given a Littlewood polynomial of the form $p(z) = \sum_{n=1}^N \xi_n z_n$ with $z_n \in \mathbb{C}$ and $|z_n| \geq 1$ for all $n$. For a universal constant $B > 0$, and an interval of radius $r$ about $0$ termed $I(r)$, we have,
    \begin{align*}
        \Pr[|p(z)| \in I(r)] \leq Crn^{-1/2}
    \end{align*}
\end{lemma}

In our case, as $|z_n| = 1$ for all $n$, we have for any fixed $w > 0$, $\widehat{\alpha}(\omega) > r$ with probability $\geq 1 - CrN^{-1/2}$. In particular, this holds for $r=1$, meaning the fourier transform of the signal is going to be a constant with many samples for any $w$. 

Therefore, with probability $\geq 1 - CN^{-1/2}$
\begin{align*}
    \left| [\mathcal{F}]\left(f(\x) - \widehat{f}(\x)\right)(\omega) \right| &= \left| \widehat{\alpha^*}(\omega) \cdot \widehat{k(\x,\cdot)}(\omega) - \left(\widehat{\alpha^*}(\omega) + \sum_{n=1}^N  \xi_n e^{-j \omega N} \right) \cdot \widehat{k(\x,\cdot)}(\omega) \right|\\
    &= \left| \left(\sum_{n=1}^N  (-\xi_n) e^{-j \omega N}\right) \cdot \widehat{k(\x,\cdot)}(\omega) \right| \\
    &\geq  \left| \widehat{k(\x,\cdot)}(\omega) \right|
\end{align*}

\section{Lower bound on error in RKHS norm}

$$\inner{\alphavec,\representers{n}}_n := \sum_{i=1}^n \alpha_i k(\x_i,\cdot) \in \Hilbert,$$

$$\inner{\inner{\alphavec,\representers{n}}_n, \inner{\betavec,\representers{n}}_n}_\Hilbert=\alphavec\T\Kmat\betavec$$

Let $f~=\inner{\alphavec^*, \representers{n}}_n$ be the regression function, and $\widehat{f}$ our estimated function on $N$ samples. So $\y=\Kmat\alphavec^*+\xi$ and $\wh\alphavec=\Kmat\inv y= \alphavec^*+\Kmat\inv \xi$.
Let $\representers{n} = (k(\cdot,\x_1),...,k(\cdot,\x_N))$. Then, using that $\widehat{f} = (\alphavec^* + \Kmat^{-1}\xi) \cdot \representers{n}$,

\begin{align*}
    \|f - \wh f\|_\Hilbert^2 &= \inner{f,f}_\Hilbert + \inner{\widehat{f},\widehat{f}}_\Hilbert - 2\inner{f,\widehat{f}}_\Hilbert \\
    &= \inner{f,f}_\Hilbert + \inner{(\alphavec^* + \Kmat^{-1}\xi)\cdot \representers{n},(\alphavec^* + \Kmat^{-1}\xi)\cdot \representers{n}}_\Hilbert - 2\inner{f,(\alphavec^* + \Kmat^{-1}\xi)\cdot \representers{n}}_\Hilbert \\
    &= \inner{f,f}_\Hilbert + \inner{f + \Kmat^{-1}\xi \cdot \representers{n},f + \Kmat^{-1}\xi \cdot \representers{n}}_\Hilbert - 2\inner{f,f + \Kmat^{-1}\xi \cdot \representers{n}}_\Hilbert \\
    &= \inner{f,f}_\Hilbert + \inner{f,f}_\Hilbert + 2\inner{f,\Kmat^{-1}\xi \cdot \representers{n}}_\Hilbert + \inner{\Kmat^{-1}\xi \cdot  \representers{n},\Kmat^{-1}\xi \cdot \representers{n}}_\Hilbert - \\
   &2\inner{f,f }_\Hilbert - 2\inner{f,\Kmat^{-1}\xi \cdot \representers{n}}_\Hilbert \\
   &= \inner{\Kmat^{-1}\xi \cdot \representers{n},\Kmat^{-1}\xi \cdot \representers{n}}_\Hilbert  \\
   &= \sum_{i_1,i_2} \xi_{i_1} \xi_{i_2} \sum_{j_1,j_2} \Kmat^{-1}_{i_1,j_1} \Kmat^{-1}_{i_2,j_2} {\Kmat_{j_1,j_2}} \\
   &=\xi \Kmat\inv\xi\\
\end{align*}

\paragraph{Remarks:} The above lower bound holds for target functions in the span of the representers of the data $\{k(\x_i,\cdot)\}$. 
However, all functions in $\mc H$ can be written as having a component in the span of $\{k(\x_i,\cdot)\}_{i=1}^n$ and perpendicular to this subspace. So this is lower bound holds for any target function via,
\begin{align*}
    \norm{f-\wh{f}}^2_\Hilbert = \norm{\Pi_n(f)-\wh{f}}_\Hilbert^2 + \norm{f-\Pi_n(f)}_\Hilbert^2
\end{align*}
where $\Pi_n:\Hilbert\rightarrow\mathrm{span}(\{k(\x_i,\cdot)\})$ is a linear projection operator.

\subsection{Concentration of Error}

We showed in the previous section that $\|f - \wh f\|_\Hilbert^2 =\xi \Kmat\inv\xi$. Let $\lambda = (\lambda_1,...,\lambda_n)$ be the ordered eigenvalues of $\Kmat \inv$. We use the Hanson-Wright (HW) inequality to bound the RHS with high probability. Note that $\Exp [\xi^T \Kmat\inv \xi] = \tr (\Kmat \inv) = \|\lambda\|_1$. Then with probability $1-\delta$, 
\begin{align*}
    \xi^T \Kmat\inv \xi &> \|\lambda\|_1 - \lambda_1 \max{} \left\{ \log(\frac{1}{\delta}),\frac{\|\lambda\|_2}{\lambda_1} \sqrt{\log(\frac{1}{\delta})}\right\} 
    % &\geq \|\lambda\|_1 - \|\lambda\|_2 \sqrt{\log(\frac{1}{\delta})}
\end{align*}









%%% Addition 4/5

\begin{theorem}
\begin{align*}
    \Exp_{\xi} \left[ \frac{1}{2\pi} \int_{0}^{2\pi} |f(t) - \hat{f}(t)|^2 \dif t \right] &\geq 1 - \sum_{n=0}^{N-1} \sum_{m \in \mathbb{Z}} \sum_{m^\prime \in \mathbb{Z}^*} \frac{\beta[mN+n]\beta[m^\prime N + n]}{\left(\sum_{k \in \mathbb{Z}} \beta[kN + n] \right)^2}
\end{align*}
\end{theorem} 
\begin{proof}
Let $x(t) = \hat{f}(t) - f(t)$. This is a periodic function in $t$ with period $2\pi$. Therefore, there exists a set of Fourier coefficients $c_k$ for $k \in \mathbb{Z}$ such that:
\begin{align}
    x(t) = \sum_{n=-\infty}^\infty c_n e^{-in 2\pi t}
\end{align}
When we measure this signal at evenly spaced points on the unit circle, we create a discrete time signal. Let $\gamma_n = \sum_{m \in \mathbb{Z}} c_{mN + n}$. Then, for $k \in \{0,...,N-1\}$,
\begin{align}
    x[k] &= \sum_{n=-\infty}^\infty c_n e^{-2\pi i \frac{nk}{N}} \\
    &= \sum_{n=0}^{N-1} \gamma_n e^{-2\pi i \frac{nk}{N}}
\end{align}
We can compute the DFT of this periodic discrete time signal.
\begin{align}
    \hat{x}[k] &= \sum_{n=0}^{N-1} x[n] e^{-2\pi i \frac{nk}{N}} \\
    &= \sum_{n=0}^{N-1} \sum_{n^\prime=0}^{N-1} \gamma_{n^\prime} e^{-2\pi i \frac{nk}{N}} e^{-2\pi i \frac{n^\prime k}{N}} \\
    &= N\gamma_k
\end{align}
Therefore, by Theorem \ref{thm:parseval_discrete},
\begin{align}
    \sum_{n=0}^{N-1} x^2[n] &= \frac{1}{N} \sum_{n=0}^{N-1} |\hat{x}[k]|^2 \\
    &= N \sum_{n=0}^{N-1} |\gamma_n|^2 \\
    &= N \sum_{n=0}^{N-1} \left|\sum_{m \in \mathbb{Z}} c_{mN + n}\right|^2 \\
    &\leq N \sum_{n=0}^{N-1} \left(\sum_{m \in \mathbb{Z}} |c_{mN + n}|\right)^2 \\
    &= N \sum_{n=-\infty}^\infty |c_n|^2 + N \sum_{n=0}^{N-1} \sum_{m \in \mathbb{Z}} \sum_{m^\prime \in \mathbb{Z}^*} |c_{mN + n} c_{m^\prime N + n}| \\
    \implies \frac{1}{N} \sum_{n=0}^{N-1} x^2[n] - &\sum_{n=0}^{N-1} \sum_{m \in \mathbb{Z}} \sum_{m^\prime \in \mathbb{Z}^*} |c_{mN + n} c_{m^\prime N + n}| \leq \sum_{n=-\infty}^\infty |c_n|^2 
\end{align}
Meanwhile, by Theorem \ref{thm:parseval_continuous},
\begin{align}
    \frac{1}{2\pi} \int_{0}^{2\pi} |x(t)|^2 \dif t &= \sum_{n=-\infty}^\infty |c_n|^2 \\
    &\geq \frac{1}{N} \sum_{n=0}^{N-1} x^2[n] - \sum_{n=0}^{N-1} \sum_{m \in \mathbb{Z}} \sum_{m^\prime \in \mathbb{Z}^*} |c_{mN + n} c_{m^\prime N + n}| \\
    &= 1 - \sum_{n=0}^{N-1} \sum_{m \in \mathbb{Z}} \sum_{m^\prime \in \mathbb{Z}^*} |c_{mN + n} c_{m^\prime N + n}|
\end{align}

We analyze the cross term in the last line here.
By lemma \ref{lemma:coeff_inspan}, 
\begin{align}
    \Exp|c_{mN+n}c_{m^\prime N + n}| &= \Exp\left|\beta[mN+n]\beta[m^\prime N + n]\right| \left|(\K\inv \xi) \cdot (e^{-i \frac{2\pi n}{N}},...,e^{-i2\pi n})\right|^2 \\
    &= \left|\beta[mN+n]\beta[m^\prime N + n]\right| \cdot \trace \left( \K^{-2} (e^{i\omega},...,e^{i\omega N})\herm (e^{-i\omega},...,e^{-i\omega N}) \right) \\
    &= \frac{\beta[mN+n]\beta[m^\prime N + n]}{\left(\sum_{k \in \mathbb{Z}} \beta[kN + n] \right)^2}
\end{align}
Finally, we derive the main theorem,
\begin{align}
    \Exp_{\xi} \left[ \frac{1}{2\pi} \int_{0}^{2\pi} |x(t)|^2 \dif t \right] &\geq 1 - \sum_{n=0}^{N-1} \sum_{m \in \mathbb{Z}} \sum_{m^\prime \in \mathbb{Z}^*} \frac{\beta[mN+n]\beta[m^\prime N + n]}{\left(\sum_{k \in \mathbb{Z}} \beta[kN + n] \right)^2}
\end{align}
\end{proof}

\section{Bandwidth}

Suppose we are in the same setting as the previous section except the kernel has a bandwidth parameter $M$ that is a multiple of $2$. In other words, the kernel is $k(x,y) = g(M(x-y) \mod 2\pi)$.

Note in this case, $g$ has period $\frac{2\pi}{M}$ and $f$ has period $\frac{2\pi}{M}$ as it lies in the span of the representers. 

\begin{lemma}
\label{lemma:coeff_inspan_M}
Let $\beta[k^\prime]$ be the $k^\prime$-th Fourier coefficient of the kernel function $g$ on the unit circle. Then for $k \in \Integer$, the Fourier coefficients of $\hat{f} - f$ satisfy 
\begin{align}
    c_k = (\K\inv \xi) \cdot (e^{-i \frac{2\pi kM}{N}},...,e^{-i 2\pi kM}) \beta[k/M] \cdot \mathbbm{1}\{k \in M \cdot \Integer\}
\end{align}
\end{lemma}
\begin{proof}
We begin by noting,
\begin{align}
    \hat{f}(x) = \sum_{i=1}^N \alpha_i k_M(x - x_i) &= \sum_{i=1}^N \alpha_i \int_{-\infty}^\infty k_M(x^\prime - x) \delta(x^\prime - x_i) dx^\prime \\
    &= \sum_{i=1}^N \int_{-\infty}^\infty k_M(x^\prime - x) \alpha(x^\prime) \delta(x^\prime - x_i) dx^\prime \\
    &= \sum_i (\alpha\delta_{x_i} * k_M)(x) 
\end{align}
Further,
\begin{align}
    f(x) = \sum_i (\alpha^* \delta_{x_i} * k)(x)
\end{align}
So, where $G_c(\omega)$ is the continuous-time fourier transform of $g(x-y) = k(x,y)$,
\begin{align}
    [\mathcal{F}](\hat{f} - f)(\omega) &= \sum_i \alpha(x_i) e^{-i\omega x_i}G_c(\omega) - \sum_i \alpha^*(x_i) e^{-i\omega x_i}G_c(\omega) \\
    &= (\alpha - \alpha^*) \cdot (e^{-i\omega x_1},...,e^{-i\omega x_N}) G_c(\omega) \\
    &= (\K\inv \xi) \cdot (e^{-i\omega x_1},...,e^{-i\omega x_N}) G_c(\omega)
\end{align}
Because $g$ is a periodic function with period $\frac{1}{M}$ (in units of time) and by Lemma \ref{lemma:kernel_unit_circle}, its Fourier transform is 
\[
    G_c(\omega) =
  \begin{cases}
        \beta[k^\prime/M] & \text{if $\omega = 2\pi k^\prime M$ for $k^\prime \in M \cdot \Integer$} \\
        0 & \text{o.w.}
  \end{cases}
\]
On the other hand,
\[
    [\mathcal{F}](\hat{f} - f)(\omega) =
  \begin{cases}
        c_k & \text{if $\omega = 2\pi k M$ for $k\in \Integer$} \\
        0 & \text{o.w.}
  \end{cases}
\]
\end{proof}

\begin{lemma}
\begin{align}
    \Exp|(\K\inv \xi) \cdot (e^{-i\omega},...,e^{-i\omega N})|^2 = \trace \left( \K^{-2} (e^{i\omega},...,e^{i\omega N})\herm (e^{-i\omega},...,e^{-i\omega N}) \right)
\end{align}
\end{lemma}
\begin{proof}
\begin{align*}
    \Exp \left[\left( \sum_{n,n^\prime} \K\inv(n,n^\prime) \xi_{n^\prime} e^{-j \omega N} \right) \left( \sum_{n,n^\prime} \K\inv(n,n^\prime) \xi_{n^\prime} e^{+j \omega N} \right)\right] &= \sum_{n^\prime}^N \sum_{n,m} K^{-1}(n,n^\prime) K^{-1}(n^\prime,m) e^{-j(n-m)w} \\ 
    &= \sum_{n,m} K^{-2}(n,m) e^{-j(n-m)w} \\
    &= \trace \left( \K^{-2} (e^{i\omega},...,e^{i\omega N})\herm (e^{-i\omega},...,e^{-i\omega N}) \right)
\end{align*}
\end{proof}

\begin{theorem}
\begin{align*}
    \Exp_{\xi} \left[ \frac{M}{2\pi} \int_{0}^{2\pi/M} |\hat{f}(t) - f(t)|^2 \dif t \right] &\geq 1 - \sum_{n=0}^{N-1} \sum_{m \in \mathbb{Z}} \sum_{m^\prime \in \mathbb{Z}^*} \frac{\beta[mN+n]\beta[m^\prime N + n]}{\left(\sum_{k \in \mathbb{Z}} \beta[kN + n] \right)^2}
\end{align*}
\end{theorem} 
\begin{proof}
Let $x(t) = \hat{f}(t) - f(t)$. Suppose $N$ is a multiple of $M$. This is a periodic function in $t$ with period $2\pi$. Therefore, there exists a set of Fourier coefficients $c_k$ for $k \in \mathbb{Z}$ such that:
\begin{align}
    x(t) = \sum_{n=-\infty}^\infty c_n e^{-in \frac{2\pi}{M} t}
\end{align}
When we measure this signal at evenly spaced points on the unit circle, we create a discrete time signal. Let $\gamma_n = \sum_{m \in \mathbb{Z}} c_{mN + n}$. Then, for $k \in \{0,...,N-1\}$,
\begin{align}
    x[k] &= \sum_{n=-\infty}^\infty c_n e^{-2\pi i \frac{nk}{MN}} \\
    &= \sum_{n=1}^{N/M} \gamma_n e^{-2\pi i \frac{nk}{MN}}
\end{align}
We can compute the DFT of this periodic discrete time signal.
\begin{align}
    \hat{x}[k] &= \sum_{n=1}^{N/M} x[n] e^{-2\pi i \frac{nk}{MN}} \\
    &= \sum_{n=1}^{N/M} \sum_{n^\prime=1}^{N/M} \gamma_{n^\prime} e^{-2\pi i \frac{nk}{MN}} e^{-2\pi i \frac{n^\prime k}{MN}} \\
    &= N\gamma_k
\end{align}
Therefore, by Theorem \ref{thm:parseval_discrete},
\begin{align}
    \sum_{n=1}^{N/M} x^2[n] &= \frac{M}{N} \sum_{n=1}^{N/M} |\hat{x}[k]|^2 \\
    &= NM \sum_{n=1}^{N/M} |\gamma_n|^2 \\
    &= NM \sum_{n=1}^{N/M} \left|\sum_{m \in \mathbb{Z}} c_{mN + n}\right|^2 \\
    &\leq NM \sum_{n=1}^{N/M} \left(\sum_{m \in \mathbb{Z}} |c_{mN + n}|\right)^2 \\
    &= NM \sum_{n=-\infty}^\infty |c_n|^2 + NM \sum_{n=1}^{N/M} \sum_{m \in \mathbb{Z}} \sum_{m^\prime \in \mathbb{Z}^*} |c_{mN + n} c_{m^\prime N + n}| \\
    \implies \frac{M}{N} \sum_{n=1}^{N/M} x^2[n] - &\sum_{n=1}^{N/M} \sum_{m \in \mathbb{Z}} \sum_{m^\prime \in \mathbb{Z}^*} |c_{mN + n} c_{m^\prime N + n}| \leq \sum_{n=-\infty}^\infty |c_n|^2 
\end{align}
Meanwhile, by Theorem \ref{thm:parseval_continuous},
\begin{align}
    \frac{M}{2\pi} \int_{0}^{2\pi/M} |x(t)|^2 \dif t &= \sum_{n=-\infty}^\infty |c_n|^2 \\
    &\geq \frac{M}{N} \sum_{n=1}^{N/M} x^2[n] - \sum_{n=1}^{N/M} \sum_{m \in \mathbb{Z}} \sum_{m^\prime \in \mathbb{Z}^*} |c_{mN/M + n} c_{m^\prime N/M + n}| \\
    &= 1 - \sum_{n=1}^{N/M} \sum_{m \in \mathbb{Z}} \sum_{m^\prime \in \mathbb{Z}^*} |c_{mN/M + n} c_{m^\prime N/M + n}|
\end{align}

We analyze the cross term in the last line here.
Let $k_1 = mN/M+n$ and $k_2 = m^\prime N/M + n$. By lemma \ref{lemma:coeff_inspan_M}, 
\begin{align}
    \Exp|c_{mN/M+n}c_{m^\prime N/M + n}| &= \mathbbm{1}\{k_1 \in M \cdot \Integer\} \mathbbm{1}\{k_2 \in M \cdot \Integer\}  \\
    &\cdot \left|\beta\left[k_1/M\right]\beta\left[k_2/M\right]\right| \Exp\left[\left|(\K\inv \xi) \cdot (e^{-i \frac{2\pi k_1 M}{N}},...,e^{-i 2\pi k_1 M})\right|\left|(\K\inv \xi) \cdot (e^{-i \frac{2\pi k_2 M}{N}},...,e^{-i 2\pi k_2 M})\right|\right]
\end{align}
For the {INSERT EXPLANATION}
\begin{align}
    &= \mathbbm{1}\{k_1 \in M \cdot \Integer\} \mathbbm{1}\{k_2 \in M \cdot \Integer\} \cdot \left|\beta\left[k_1/M\right]\beta\left[k_2/M\right]\right| \Exp \left|(\K\inv \xi) \cdot (e^{-i \frac{2\pi n M}{N}},...,e^{-i 2\pi n M})\right|^2 \\
    &= \mathbbm{1}\{k_1 \in M \cdot \Integer\} \mathbbm{1}\{k_2 \in M \cdot \Integer\}
    \cdot \left|\beta\left[k_1/M\right]\beta\left[k_2/M\right]\right| \cdot \trace \left( \K^{-2} (e^{i \frac{2\pi n M}{N}},...,e^{i 2\pi n M} )\herm (e^{i \frac{2\pi n M}{N}},...,e^{i 2\pi n M}) \right) \\
    &=  \frac{\mathbbm{1}\{k_1 \in M \cdot \Integer\} \mathbbm{1}\{k_2 \in M \cdot \Integer\}
    \cdot \left|\beta\left[k_1/M\right]\beta\left[k_2/M\right]\right|}{COMPUTE \quad DENOMINATOR}
\end{align}
Finally, we derive the main theorem,
\begin{align}
    \Exp_{\xi} \left[ \frac{M}{2\pi} \int_{0}^{2\pi/M} |x(t)|^2 \dif t \right] &\geq 1 - \sum_{n=0}^{N-1} \sum_{m \in \mathbb{Z}} \sum_{m^\prime \in \mathbb{Z}^*} \frac{\beta[mN+n]\beta[m^\prime N + n]}{\left(\sum_{k \in \mathbb{Z}} \beta[kN + n] \right)^2}
\end{align}
\end{proof}





%%% 4/7
%Old proofs from Inconsistency section

So, where $G_c(\omega)$ is the continuous-time fourier transform of $g(x-y) = k(x,y)$,
\begin{align}
    [\mathcal{F}](\hat{f} - f)(\omega) &= \sum_i \alpha(x_i) e^{-i\omega x_i}G_c(\omega) - \sum_i \alpha^*(x_i) e^{-i\omega x_i}G_c(\omega) \\
    &= (\alpha - \alpha^*) \cdot (e^{-i\omega x_1},...,e^{-i\omega x_N}) G_c(\omega) \\
    &= (\K\inv \xi) \cdot (e^{-i\omega x_1},...,e^{-i\omega x_N}) G_c(\omega)
\end{align}
Because $g$ is a periodic function with period $2\pi$, its Fourier transform is 
\[
    G_c(\omega) =
  \begin{cases}
        \beta^M[k] & \text{if $\omega = 2\pi k $ for $k \in \Integer$} \\
        0 & \text{o.w.}
  \end{cases}
\]
Similarly,
\[
    [\mathcal{F}](\hat{f} - f)(\omega) =
  \begin{cases}
        c_k & \text{if $\omega = 2\pi k $ for $k \in \Integer$} \\
        0 & \text{o.w.}
  \end{cases}
\]


\begin{theorem}[Discrete Parseval's Theorem]
\label{thm:parseval_discrete}
For a discrete signal $x[k]$ with period $N$ and DFT $\hat{x}$,
\begin{align*}
    \sum_{n=0}^{N-1} |x[n]|^2 = \frac{1}{N}\sum_{n=0}^{N-1} |\hat{x}[n]|^2
\end{align*}
\end{theorem}
